# Supplementary material for: A Unified Framework for Lifted Training and Inversion Approaches
Source: arXiv:2510.09796 source file (2026-02-06)
Supplement: Supplementary file 2 [file appendix02.tex]

\begin{frontmatter}
\chapter{Appendix title}%\label{chap:appb}
\end{frontmatter}
